# Supplementary material for: Trade-offs between structural richness and perceptual robustness in music network representations
Source: arXiv:2509.14053 source file (2026-07-26)
Supplement: Supplementary file 1 [file SI.pdf]

# Supplementary Information for “Network representations reveal structured uncertainty in music”

Lluc Bono Rosselló,<sup>1</sup> Robert Jankowski,<sup>2,3</sup> Hugues Bersini,<sup>1</sup> Marián Boguñá,<sup>2,3</sup> and M. Ángeles Serrano<sup>2,3,4</sup>

<sup>1</sup>*Institute for Interdisciplinary Studies on Artificial Intelligence (IRIDIA),  
Université Libre de Bruxelles, Brussels, Belgium*

<sup>2</sup>*Departament de Física de la Matèria Condensada,  
Universitat de Barcelona, Martí i Franquès 1, E-08028 Barcelona, Spain*

<sup>3</sup>*Universitat de Barcelona Institute of Complex Systems (UBICS), Universitat de Barcelona, Barcelona, Spain*

<sup>4</sup>*ICREA, Passeig Lluís Companys 23, E-08010 Barcelona, Spain*

(Dated: September 17, 2025)

## CONTENTS

|                                           |    |
|-------------------------------------------|----|
| I. Descriptive analysis of the datasets   | 2  |
| II. Network properties                    | 5  |
| III. Entropy in music networks            | 11 |
| IV. KL divergence in music network models | 12 |

# I. DESCRIPTIVE ANALYSIS OF THE DATASETS

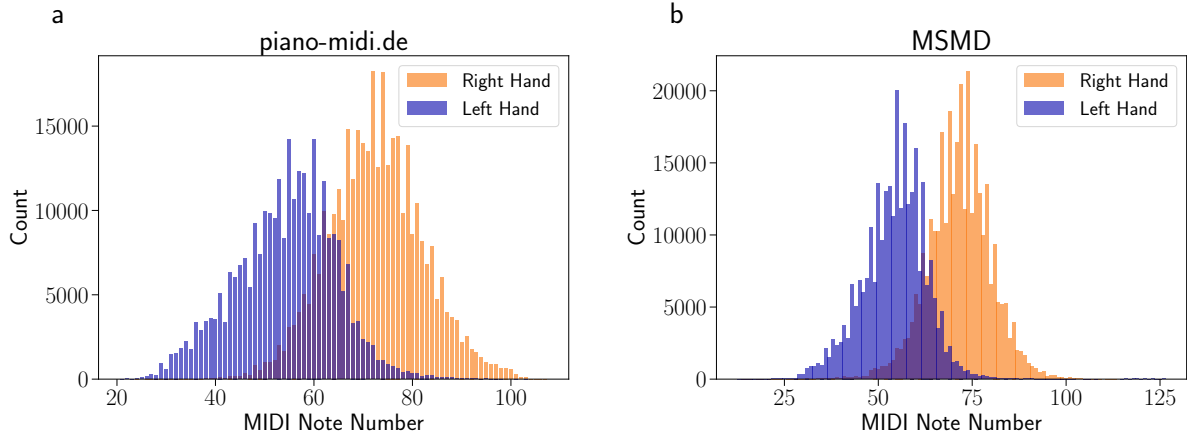

FIG. S1: The distribution of the MIDI note number for (a) piano-midi.de and (b) MSMD datasets.

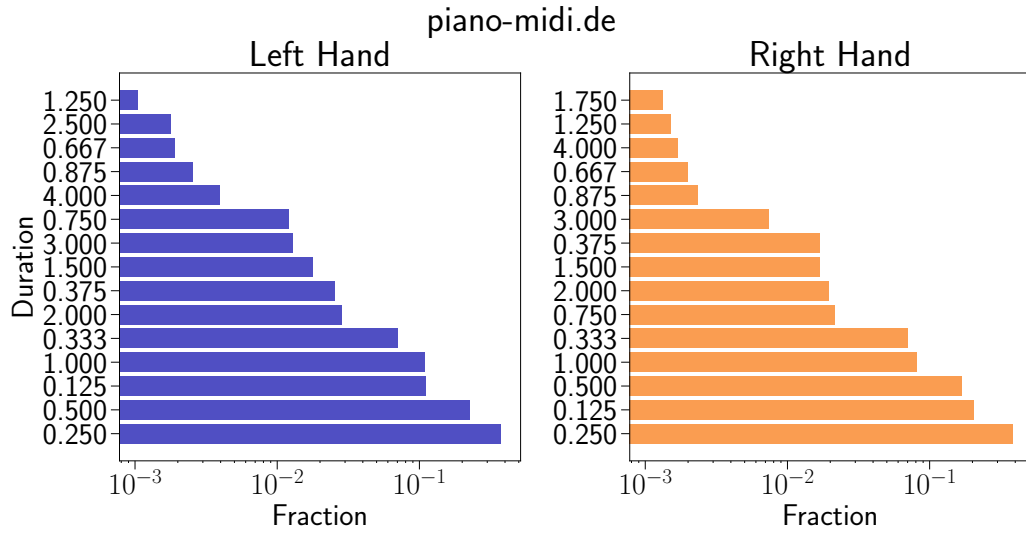

FIG. S2: Top 15 most frequent durations for the left and right hand parts from the piano-midi.de dataset.

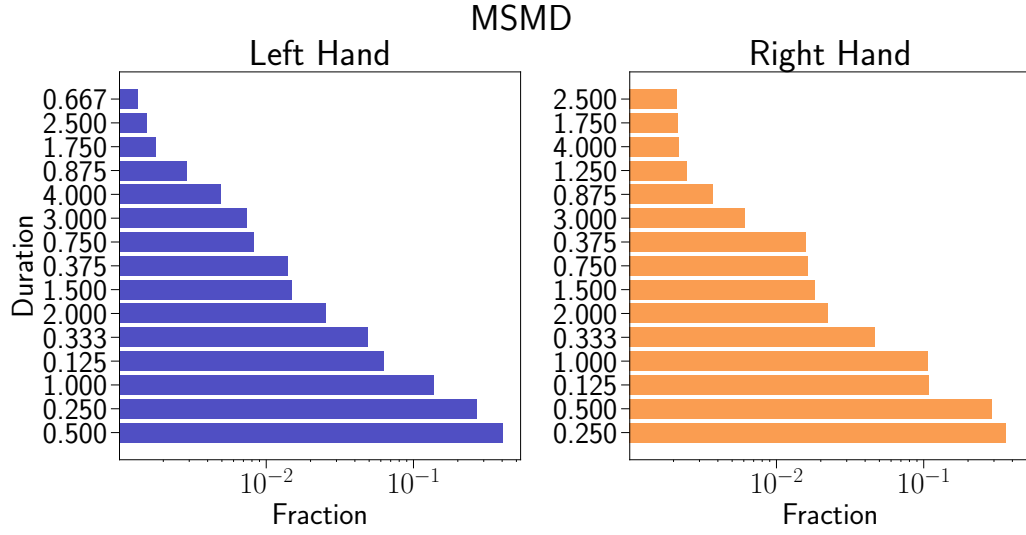

FIG. S3: Top 15 most frequent durations for the left and right hand parts from the MSMD dataset.

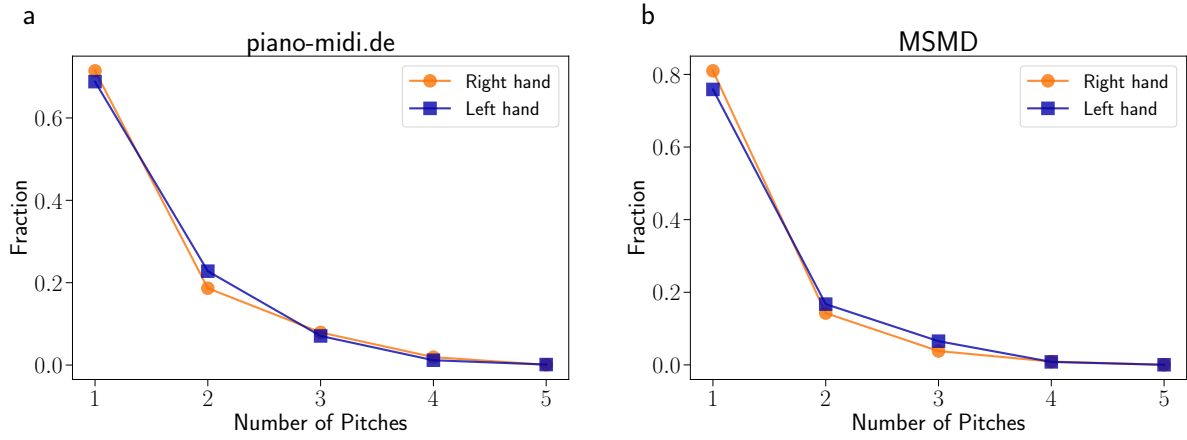

FIG. S4: Fraction of number of pitches for left and right hand for (a) piano-midi.de and (b) MSMD datasets.

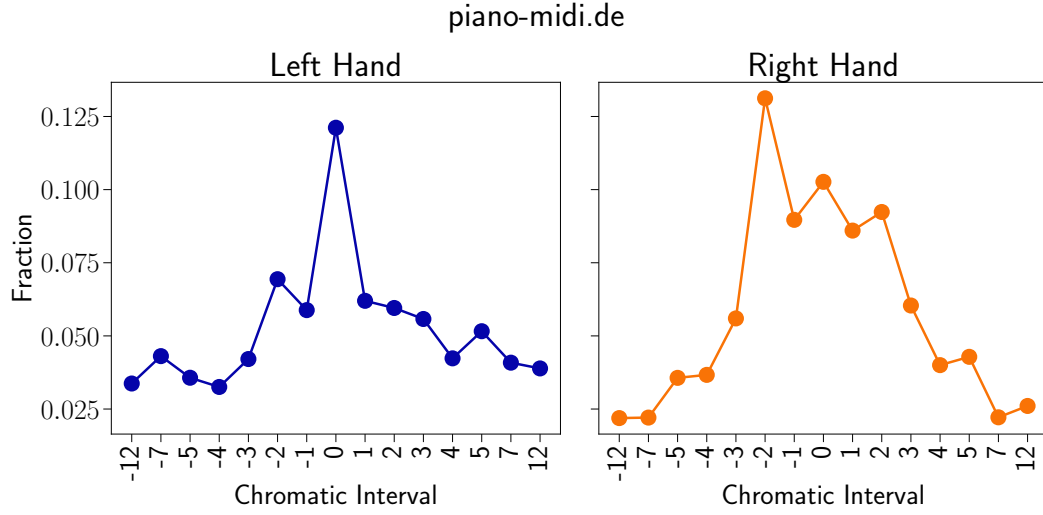

FIG. S5: Top 15 most frequent chromatic intervals for the left and right hand parts from the piano-midi.de dataset.

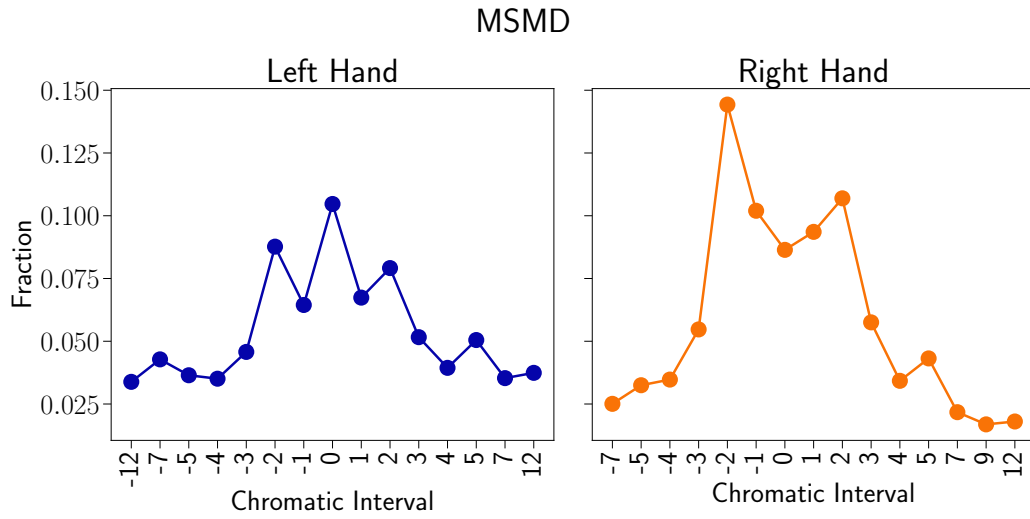

FIG. S6: Top 15 most frequent chromatic intervals for the left and right hand parts from the MSMD dataset.

## II. NETWORK PROPERTIES

TABLE S1: **Network metrics averaged by model.** Size  $N$ , number of edges  $E$ , average degree  $\langle k \rangle$ , reciprocity  $r$ , weighted reciprocity  $r_w$ , number of self-loops  $\#$  loops, average undirected and unweighted clustering coefficient  $\langle C \rangle$ , average directed and weighted clustering coefficient  $\langle C_d \rangle$ , average undirected and weighted clustering coefficient  $\langle C_w \rangle$ , average directed and weighted clustering coefficient  $\langle C_{d,w} \rangle$ , average out-degree  $\langle k_{out} \rangle$ , degree heterogeneity  $\langle k^2 \rangle / \langle k \rangle^2$ , average in-strength  $\langle s_{in} \rangle$ , average shortest path length  $\langle l \rangle$ , closeness centrality  $CC$ , betweenness centrality  $BC$ , weighted entropy  $S$  and weighted KL-divergence, across different models averaged over all music pieces for the right hand.

| Model                                       | Duration          | Interval           | Pitch               | Pitch+Duration      | Pitch+Octave        | Pitch+Octave+Duration | Pitch+Octave(split) | Pitch(split)        |
|---------------------------------------------|-------------------|--------------------|---------------------|---------------------|---------------------|-----------------------|---------------------|---------------------|
| $N$                                         | $9.04 \pm 3.40$   | $26.40 \pm 9.06$   | $30.28 \pm 21.07$   | $72.95 \pm 54.16$   | $64.66 \pm 64.09$   | $118.77 \pm 110.25$   | $28.34 \pm 12.08$   | $10.99 \pm 1.49$    |
| $E$                                         | $30.83 \pm 17.14$ | $132.35 \pm 81.58$ | $128.82 \pm 103.53$ | $222.66 \pm 191.07$ | $211.85 \pm 201.21$ | $279.73 \pm 264.41$   | $253.26 \pm 233.70$ | $84.62 \pm 33.11$   |
| $\langle k \rangle$                         | $6.50 \pm 1.51$   | $9.33 \pm 3.12$    | $8.46 \pm 2.28$     | $5.95 \pm 1.82$     | $6.89 \pm 2.29$     | $4.76 \pm 1.49$       | $15.39 \pm 7.56$    | $14.97 \pm 4.68$    |
| $r$                                         | $0.57 \pm 0.13$   | $0.44 \pm 0.11$    | $0.53 \pm 0.14$     | $0.30 \pm 0.14$     | $0.43 \pm 0.14$     | $0.26 \pm 0.14$       | $0.62 \pm 0.10$     | $0.77 \pm 0.09$     |
| $r_w$                                       | $0.29 \pm 0.14$   | $0.41 \pm 0.11$    | $0.51 \pm 0.16$     | $0.32 \pm 0.17$     | $0.43 \pm 0.16$     | $0.28 \pm 0.16$       | $0.58 \pm 0.11$     | $0.65 \pm 0.11$     |
| $\#$ loops                                  | $3.99 \pm 1.66$   | $4.71 \pm 2.42$    | $10.81 \pm 9.45$    | $8.67 \pm 10.33$    | $13.17 \pm 15.77$   | $8.39 \pm 11.70$      | $13.75 \pm 10.54$   | $7.99 \pm 3.01$     |
| $\langle C \rangle$                         | $0.65 \pm 0.17$   | $0.47 \pm 0.13$    | $0.49 \pm 0.18$     | $0.26 \pm 0.13$     | $0.34 \pm 0.15$     | $0.19 \pm 0.10$       | $0.62 \pm 0.11$     | $0.84 \pm 0.10$     |
| $\langle C_d \rangle$                       | $0.58 \pm 0.17$   | $0.35 \pm 0.12$    | $0.42 \pm 0.17$     | $0.19 \pm 0.11$     | $0.27 \pm 0.13$     | $0.13 \pm 0.08$       | $0.52 \pm 0.12$     | $0.79 \pm 0.12$     |
| $\langle C_w \rangle$                       | $0.03 \pm 0.04$   | $0.06 \pm 0.04$    | $0.09 \pm 0.06$     | $0.05 \pm 0.04$     | $0.06 \pm 0.05$     | $0.04 \pm 0.03$       | $0.09 \pm 0.05$     | $0.16 \pm 0.07$     |
| $\langle C_{d,w} \rangle$                   | $0.03 \pm 0.03$   | $0.04 \pm 0.03$    | $0.07 \pm 0.05$     | $0.03 \pm 0.03$     | $0.05 \pm 0.03$     | $0.02 \pm 0.02$       | $0.07 \pm 0.04$     | $0.15 \pm 0.06$     |
| $\langle k_{out} \rangle$                   | $3.25 \pm 0.76$   | $4.67 \pm 1.56$    | $4.23 \pm 1.14$     | $2.97 \pm 0.91$     | $3.45 \pm 1.15$     | $2.38 \pm 0.74$       | $7.70 \pm 3.78$     | $7.49 \pm 2.34$     |
| $\langle k^2 \rangle / \langle k \rangle^2$ | $1.39 \pm 0.19$   | $1.54 \pm 0.19$    | $1.63 \pm 0.32$     | $1.83 \pm 0.40$     | $1.74 \pm 0.37$     | $1.74 \pm 0.39$       | $1.35 \pm 0.11$     | $1.11 \pm 0.08$     |
| $\langle s_{in} \rangle$                    | $72.66 \pm 60.96$ | $20.59 \pm 16.36$  | $20.76 \pm 17.33$   | $8.40 \pm 7.33$     | $10.26 \pm 7.00$    | $5.25 \pm 3.30$       | $35.96 \pm 32.49$   | $107.96 \pm 134.90$ |
| $\langle l \rangle$                         | $1.80 \pm 0.27$   | $2.32 \pm 0.27$    | $2.64 \pm 0.74$     | $4.12 \pm 1.29$     | $4.08 \pm 1.88$     | $6.31 \pm 3.24$       | $2.11 \pm 0.36$     | $1.36 \pm 0.20$     |
| $CC$                                        | $0.19 \pm 0.10$   | $0.27 \pm 0.08$    | $0.23 \pm 0.08$     | $0.18 \pm 0.07$     | $0.19 \pm 0.09$     | $0.14 \pm 0.07$       | $0.30 \pm 0.09$     | $0.26 \pm 0.11$     |
| $BC$                                        | $0.20 \pm 0.06$   | $0.08 \pm 0.03$    | $0.10 \pm 0.04$     | $0.07 \pm 0.04$     | $0.08 \pm 0.05$     | $0.07 \pm 0.05$       | $0.07 \pm 0.04$     | $0.12 \pm 0.03$     |
| $S$                                         | $1.23 \pm 0.40$   | $2.27 \pm 0.46$    | $2.29 \pm 0.44$     | $1.91 \pm 0.58$     | $2.05 \pm 0.52$     | $1.57 \pm 0.57$       | $2.80 \pm 0.62$     | $2.60 \pm 0.39$     |
| $D_{KL}$                                    | $0.23 \pm 0.15$   | $0.89 \pm 0.23$    | $0.73 \pm 0.27$     | $1.35 \pm 0.35$     | $1.10 \pm 0.29$     | $1.58 \pm 0.29$       | $0.67 \pm 0.20$     | $0.31 \pm 0.17$     |

TABLE S2: **Network metrics averaged by model.** Topological properties across different models averaged over all music pieces for the left hand. See Table S1 for more details.

| Model                                       | Duration          | Interval           | Pitch             | Pitch+Duration      | Pitch+Octave        | Pitch+Octave+Duration | Pitch+Octave(split) | Pitch(split)       |
|---------------------------------------------|-------------------|--------------------|-------------------|---------------------|---------------------|-----------------------|---------------------|--------------------|
| $N$                                         | $8.47 \pm 3.46$   | $29.15 \pm 11.12$  | $25.69 \pm 18.4$  | $58.16 \pm 47.76$   | $53.79 \pm 49.44$   | $94.99 \pm 91.08$     | $29.1 \pm 12.3$     | $10.81 \pm 1.62$   |
| $E$                                         | $27.74 \pm 16.02$ | $124.51 \pm 87.99$ | $106.3 \pm 88.39$ | $174.46 \pm 157.25$ | $174.65 \pm 167.35$ | $215.4 \pm 206.98$    | $230.63 \pm 225.19$ | $76.38 \pm 32.91$  |
| $\langle k \rangle$                         | $6.28 \pm 1.45$   | $7.84 \pm 2.87$    | $8.16 \pm 2.45$   | $5.87 \pm 1.81$     | $6.45 \pm 2.12$     | $4.53 \pm 1.3$        | $13.56 \pm 7.06$    | $13.68 \pm 4.68$   |
| $r$                                         | $0.56 \pm 0.13$   | $0.36 \pm 0.11$    | $0.53 \pm 0.16$   | $0.33 \pm 0.14$     | $0.41 \pm 0.15$     | $0.27 \pm 0.14$       | $0.57 \pm 0.12$     | $0.73 \pm 0.11$    |
| $r_w$                                       | $0.26 \pm 0.14$   | $0.32 \pm 0.14$    | $0.49 \pm 0.17$   | $0.35 \pm 0.18$     | $0.42 \pm 0.18$     | $0.3 \pm 0.18$        | $0.54 \pm 0.14$     | $0.6 \pm 0.12$     |
| # loops                                     | $4.09 \pm 1.69$   | $4.23 \pm 2.52$    | $10.26 \pm 9.67$  | $9.79 \pm 11.24$    | $11.05 \pm 14.7$    | $7.94 \pm 12.39$      | $11.89 \pm 10.3$    | $7.55 \pm 3.01$    |
| $\langle C \rangle$                         | $0.64 \pm 0.18$   | $0.39 \pm 0.13$    | $0.5 \pm 0.19$    | $0.28 \pm 0.14$     | $0.32 \pm 0.15$     | $0.18 \pm 0.11$       | $0.57 \pm 0.11$     | $0.82 \pm 0.11$    |
| $\langle C_d \rangle$                       | $0.56 \pm 0.18$   | $0.27 \pm 0.11$    | $0.43 \pm 0.18$   | $0.2 \pm 0.12$      | $0.24 \pm 0.13$     | $0.12 \pm 0.08$       | $0.48 \pm 0.12$     | $0.76 \pm 0.13$    |
| $\langle C_w \rangle$                       | $0.03 \pm 0.03$   | $0.05 \pm 0.04$    | $0.09 \pm 0.07$   | $0.05 \pm 0.05$     | $0.06 \pm 0.05$     | $0.04 \pm 0.04$       | $0.08 \pm 0.05$     | $0.14 \pm 0.07$    |
| $\langle C_{d,w} \rangle$                   | $0.03 \pm 0.03$   | $0.03 \pm 0.02$    | $0.08 \pm 0.06$   | $0.04 \pm 0.03$     | $0.04 \pm 0.04$     | $0.02 \pm 0.02$       | $0.07 \pm 0.04$     | $0.13 \pm 0.06$    |
| $\langle k_{out} \rangle$                   | $3.14 \pm 0.72$   | $3.92 \pm 1.44$    | $4.08 \pm 1.23$   | $2.93 \pm 0.9$      | $3.22 \pm 1.06$     | $2.26 \pm 0.65$       | $6.78 \pm 3.53$     | $6.84 \pm 2.34$    |
| $\langle k^2 \rangle / \langle k \rangle^2$ | $1.35 \pm 0.18$   | $1.57 \pm 0.24$    | $1.58 \pm 0.33$   | $1.72 \pm 0.34$     | $1.65 \pm 0.34$     | $1.62 \pm 0.32$       | $1.4 \pm 0.13$      | $1.14 \pm 0.11$    |
| $\langle s_{in} \rangle$                    | $70.9 \pm 56.98$  | $15.08 \pm 12.2$   | $18.63 \pm 13.11$ | $8.3 \pm 5.39$      | $9.14 \pm 5.52$     | $5.27 \pm 3.31$       | $30.7 \pm 31.75$    | $93.74 \pm 121.57$ |
| $\langle l \rangle$                         | $1.81 \pm 0.32$   | $2.59 \pm 0.41$    | $2.53 \pm 0.74$   | $3.94 \pm 1.31$     | $3.82 \pm 1.35$     | $5.99 \pm 2.63$       | $2.2 \pm 0.35$      | $1.42 \pm 0.21$    |
| $CC$                                        | $0.2 \pm 0.1$     | $0.24 \pm 0.08$    | $0.24 \pm 0.09$   | $0.19 \pm 0.08$     | $0.19 \pm 0.09$     | $0.14 \pm 0.07$       | $0.3 \pm 0.09$      | $0.27 \pm 0.11$    |
| $BC$                                        | $0.22 \pm 0.06$   | $0.09 \pm 0.04$    | $0.11 \pm 0.05$   | $0.09 \pm 0.06$     | $0.09 \pm 0.06$     | $0.09 \pm 0.06$       | $0.07 \pm 0.04$     | $0.12 \pm 0.03$    |
| $S$                                         | $1.1 \pm 0.4$     | $1.97 \pm 0.52$    | $2.16 \pm 0.49$   | $1.81 \pm 0.53$     | $1.88 \pm 0.54$     | $1.43 \pm 0.51$       | $2.65 \pm 0.63$     | $2.47 \pm 0.4$     |
| $D_{KL}$                                    | $0.23 \pm 0.14$   | $1.1 \pm 0.27$     | $0.69 \pm 0.26$   | $1.23 \pm 0.32$     | $1.16 \pm 0.27$     | $1.52 \pm 0.29$       | $0.76 \pm 0.25$     | $0.33 \pm 0.17$    |

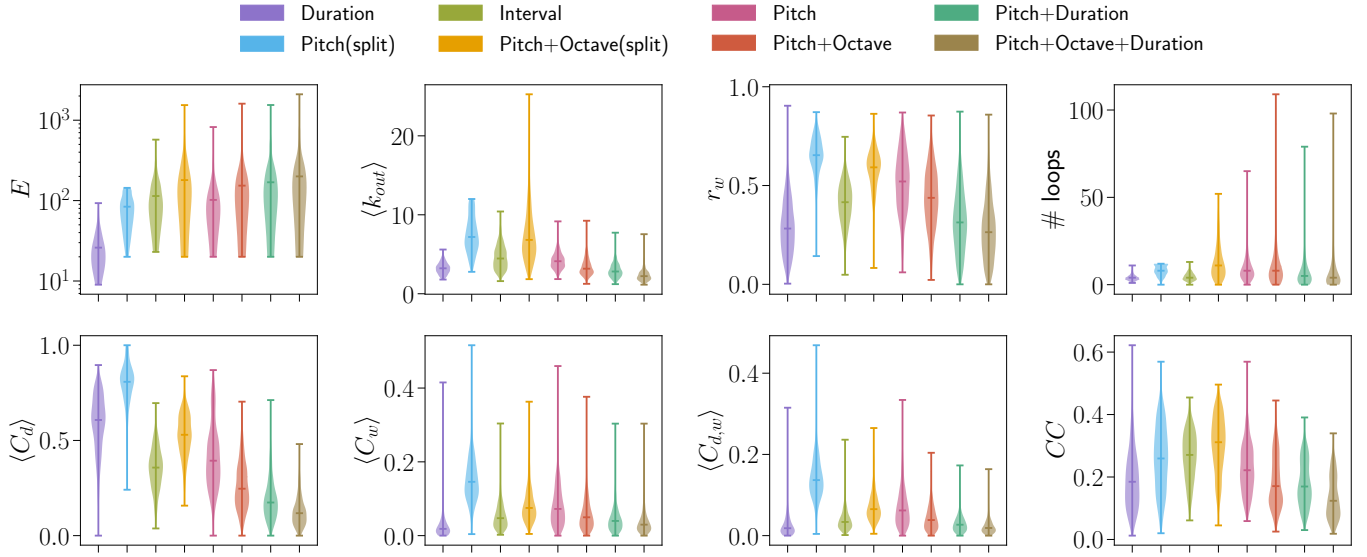

FIG. S7: Violin plots showing the distribution of eight network measures— number of edges  $E$ , average out-degree  $\langle k_{out} \rangle$ , weighted reciprocity  $r_w$ , number of self-loops # loops, average directed and weighted clustering coefficient  $\langle C_d \rangle$ , average undirected and weighted clustering coefficient  $\langle C_w \rangle$ , average directed and weighted clustering coefficient  $\langle C_{d,w} \rangle$ , and closeness centrality  $CC$ —across different models averaged over all music pieces for the **right** hand. Each color corresponds to a specific model, with the models sorted by their mean network size ( $N$ ). A solid line within each violin indicates the median of each distribution.

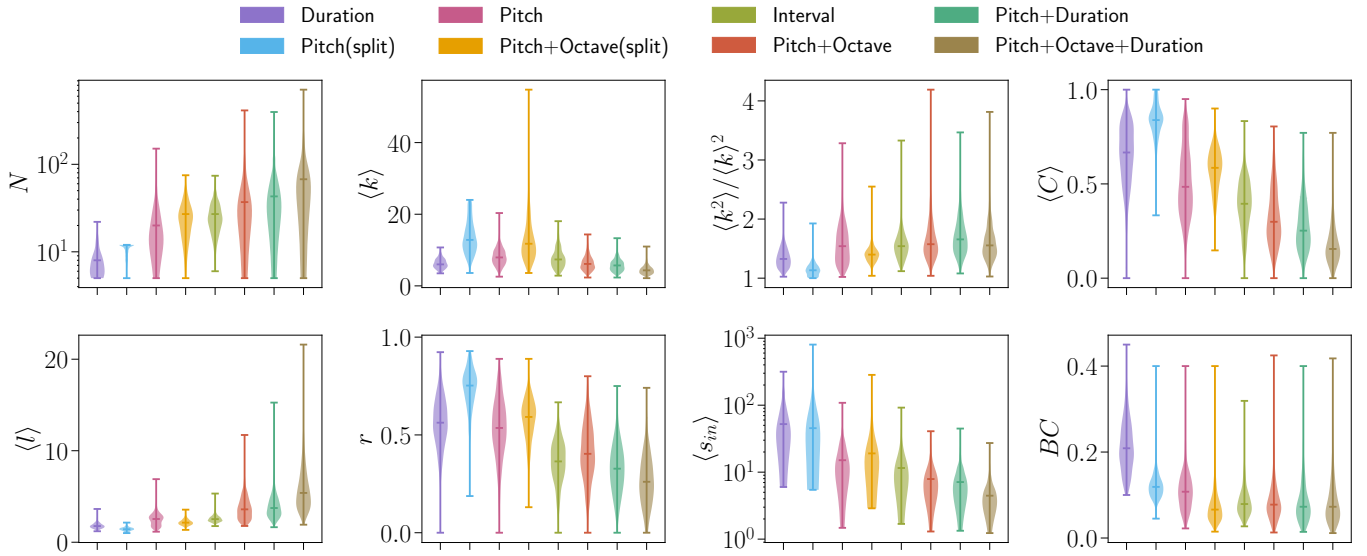

FIG. S8: Violin plots showing the distribution of eight network measures: size  $N$ , average degree  $\langle k \rangle$ , degree heterogeneity  $\langle k^2 \rangle / \langle k \rangle^2$ , average clustering coefficient  $\langle C \rangle$ , average shortest path length  $\langle l \rangle$ , reciprocity  $r$ , average in-strength  $\langle s_{in} \rangle$ , and betweenness centrality  $BC$ , across different models averaged over all music pieces for the **left** hand. Each color corresponds to a specific model, with the models sorted by their mean network size ( $N$ ). A solid line within each violin indicates the median of each distribution.



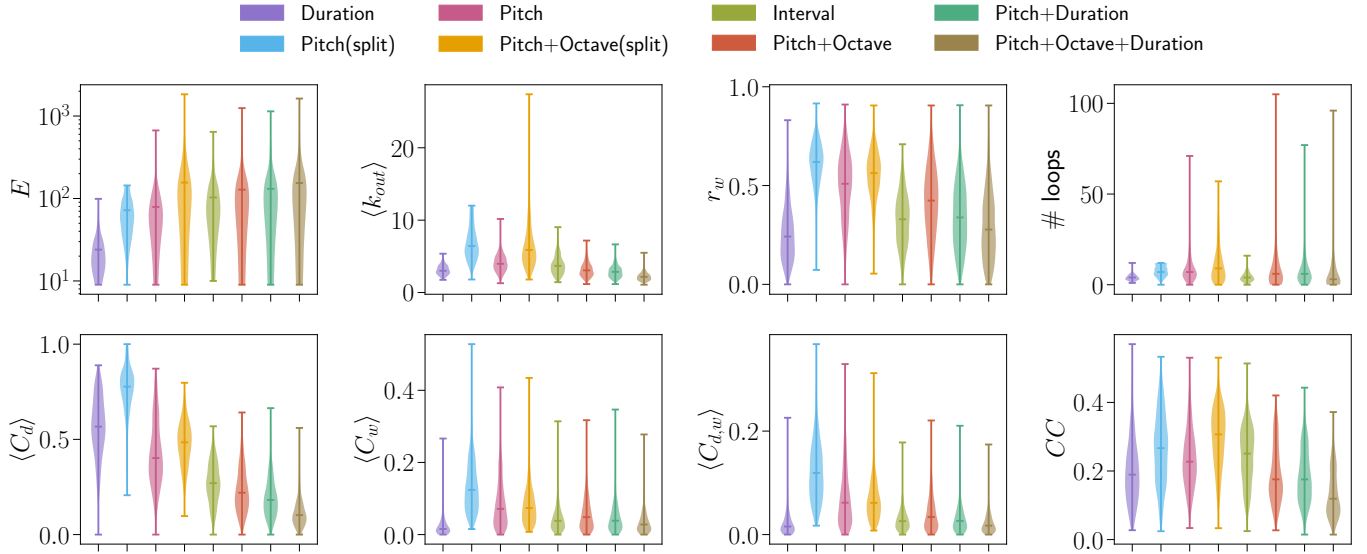

FIG. S9: Violin plots showing the distribution of eight network measures— number of edges  $E$ , average out-degree  $\langle k_{out} \rangle$ , weighted reciprocity  $r_w$ , number of self-loops  $\# \text{ loops}$ , average directed and weighted clustering coefficient  $\langle C_d \rangle$ , average undirected and weighted clustering coefficient  $\langle C_w \rangle$ , average directed and weighted clustering coefficient  $\langle C_{d,w} \rangle$ , and closeness centrality  $CC$ —across different models averaged over all music pieces for the **left** hand. Each color corresponds to a specific model, with the models sorted by their mean network size ( $N$ ). A solid line within each violin indicates the median of each distribution.

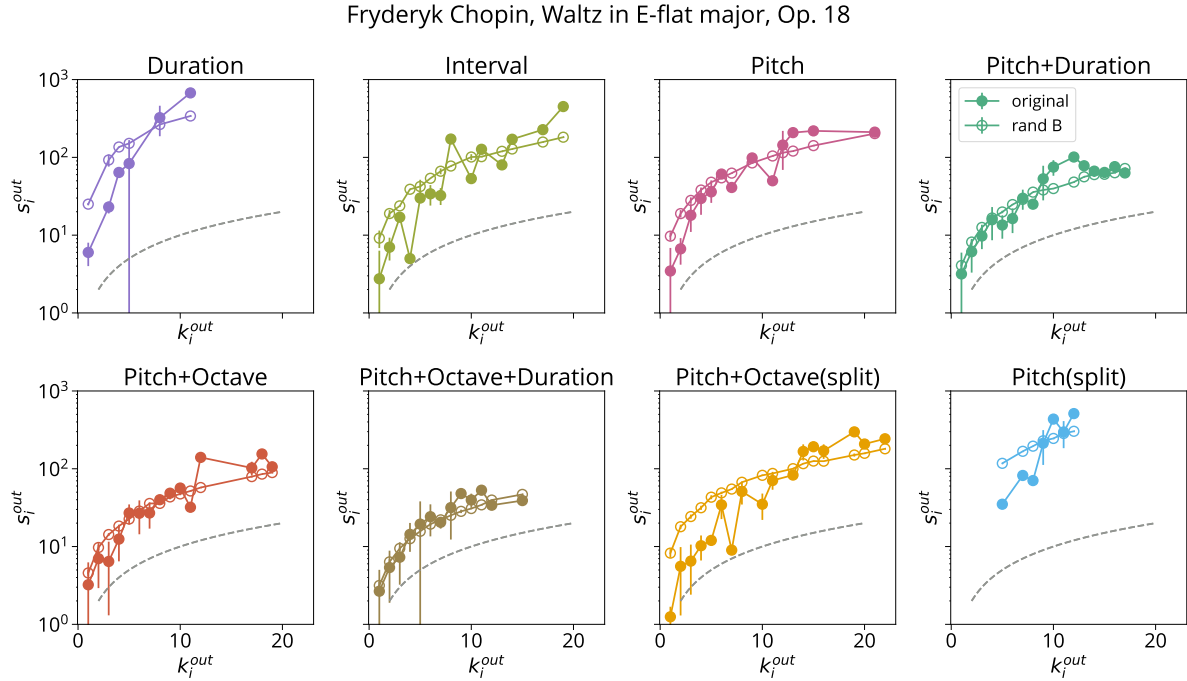

FIG. S10: The relationship between the out-degree  $k_i^{out}$  and the out-strength  $s_i^{out}$  for eight different network music representations. The out-strength values are averaged over each out-degree class. The empty symbols correspond to the randomized network (*Rand B*) when we shuffle the edge weights keeping the skeleton of the network.

## Mendelssohn Op. 30 No. 5

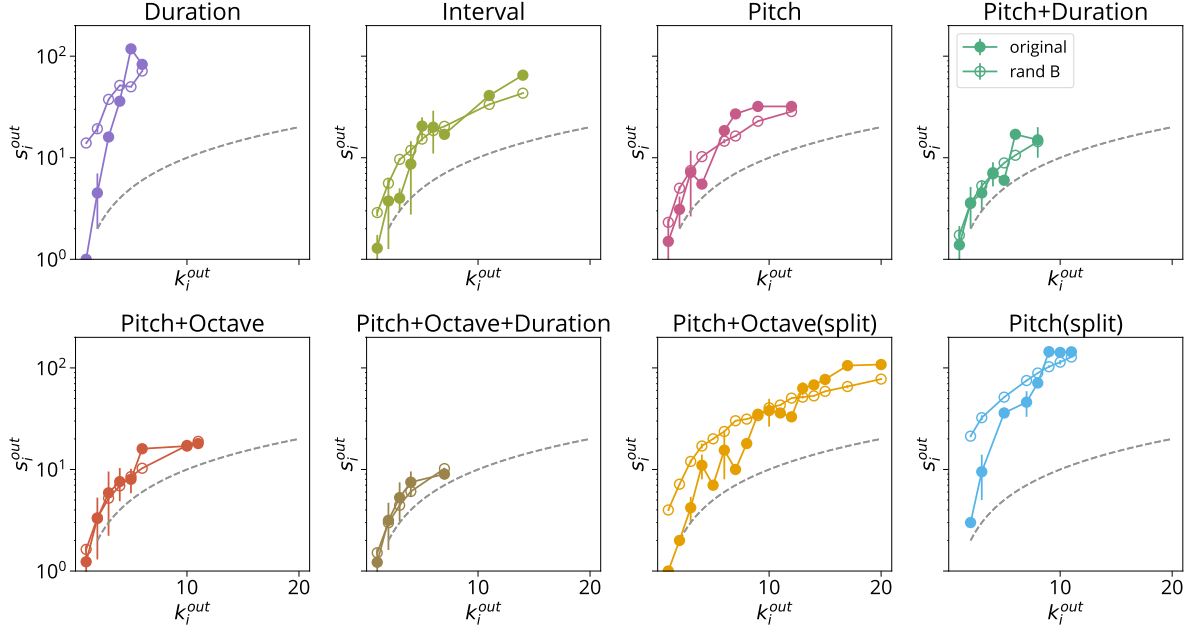

FIG. S11: The relationship between the out-degree  $k_i^{\text{out}}$  and the out-strength  $s_i^{\text{out}}$  for eight different network music representations. The out-strength values are averaged over each out-degree class. The empty symbols correspond to the randomized network (*Rand B*) when we shuffle the edge weights keeping the skeleton of the network.

## Haydn's Symphony No. 43 in E-flat major

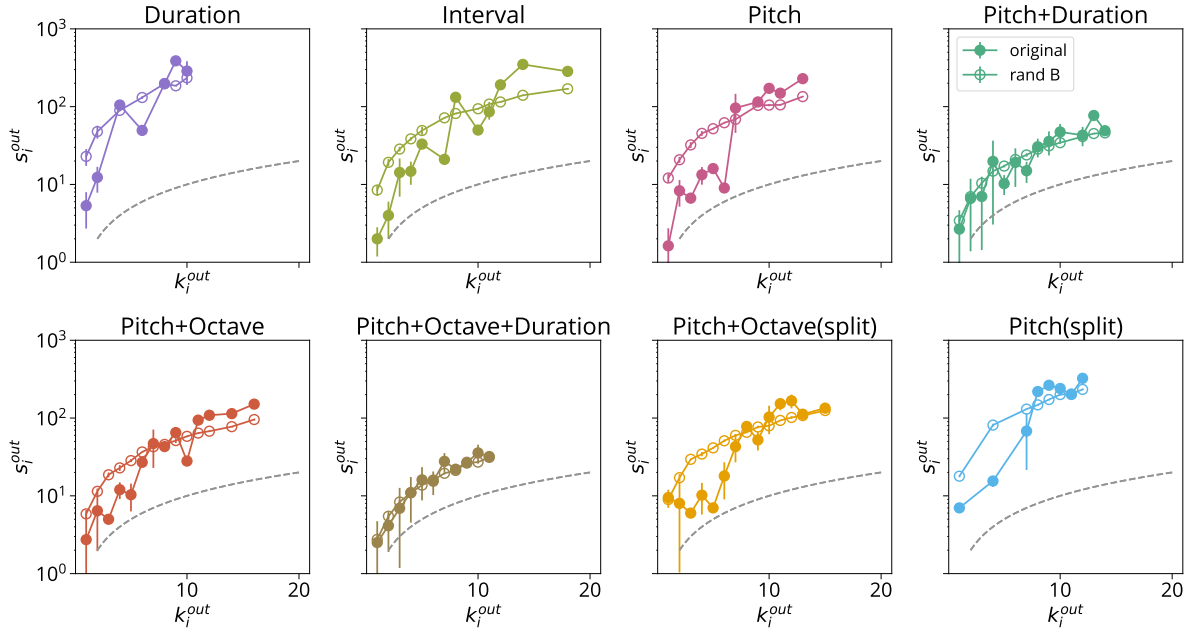

FIG. S12: The relationship between the out-degree  $k_i^{\text{out}}$  and the out-strength  $s_i^{\text{out}}$  for eight different network music representations. The out-strength values are averaged over each out-degree class. The empty symbols correspond to the randomized network (*Rand B*) when we shuffle the edge weights keeping the skeleton of the network.

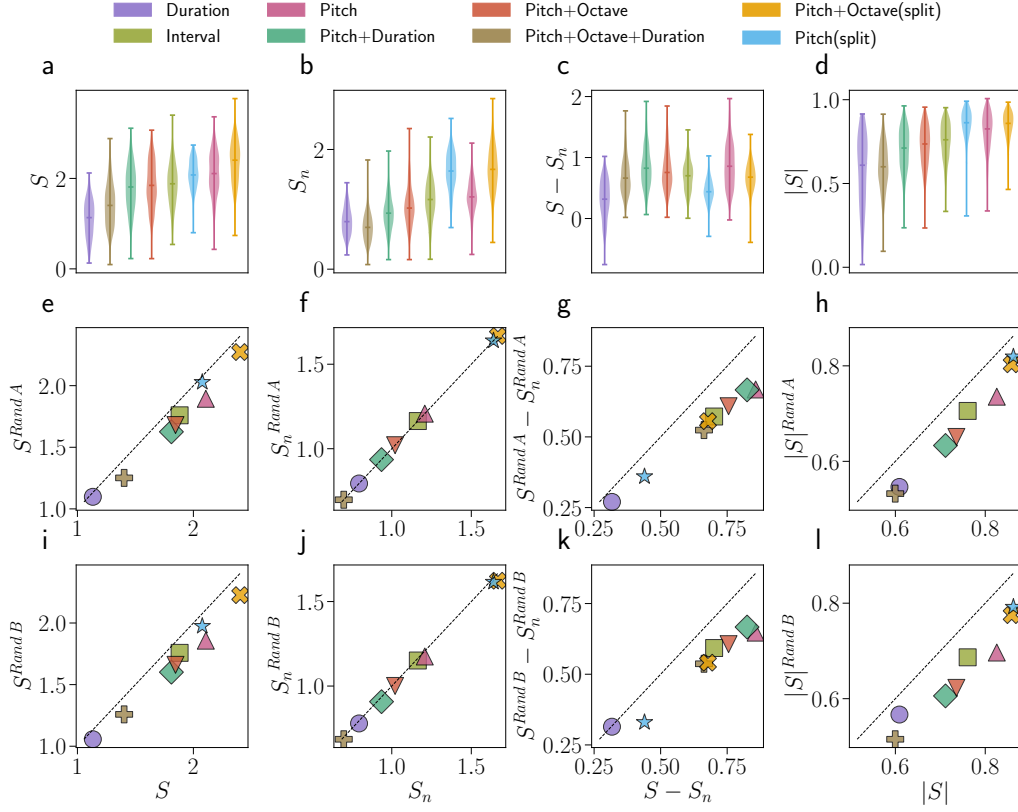

FIG. S13: Violin plots illustrating the distribution of (a) weighted entropy  $S$ , (b) average node weighted entropy  $S_n$ , (c) difference between weighted entropy and average node weighted entropy  $S - S_n$ , (d) normalized weighted entropy  $|S|$  for each network model. Each violin is color-coded by model, and the models are sorted by their mean weighted entropy ( $S$ ). The median of each distribution is indicated by a solid line within the violin. (e–l) The relationships between the median value of the original and randomized entropies. Two rows correspond to two types of network randomization (A and B). Here, we plot values for the left hand.

### III. ENTROPY IN MUSIC NETWORKS

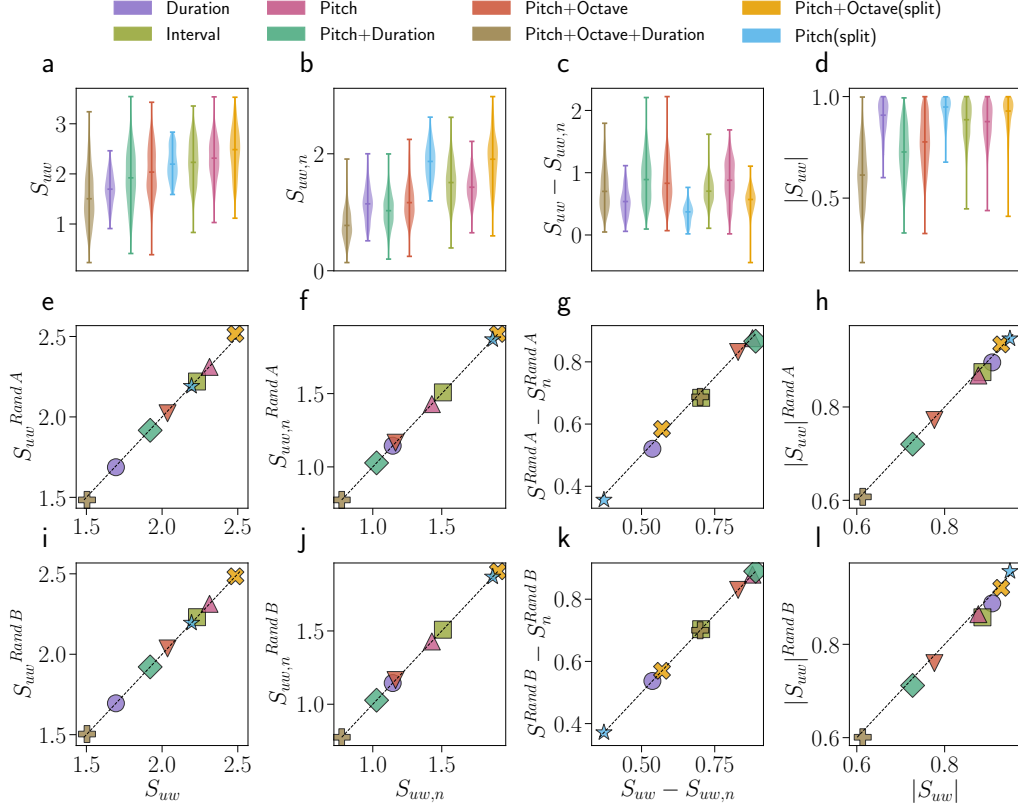

FIG. S14: Violin plots illustrating the distribution of (a) unweighted entropy  $S_{uw}$ , (b) average node unweighted entropy  $S_{uw,n}$ , (c) difference between unweighted entropy and average node unweighted entropy  $S_{uw} - S_{uw,n}$ , (d) normalized unweighted entropy  $|S_{uw}|$  for each network model. Each violin is color-coded by model, and the models are sorted by their mean unweighted entropy ( $S_{uw}$ ). The median of each distribution is indicated by a solid line within the violin. (e–l) The relationships between the median value of the original and randomized entropies. Two rows correspond to two types of network randomization (A and B). Here, we plot values for the right hand.

#### IV. KL DIVERGENCE IN MUSIC NETWORK MODELS

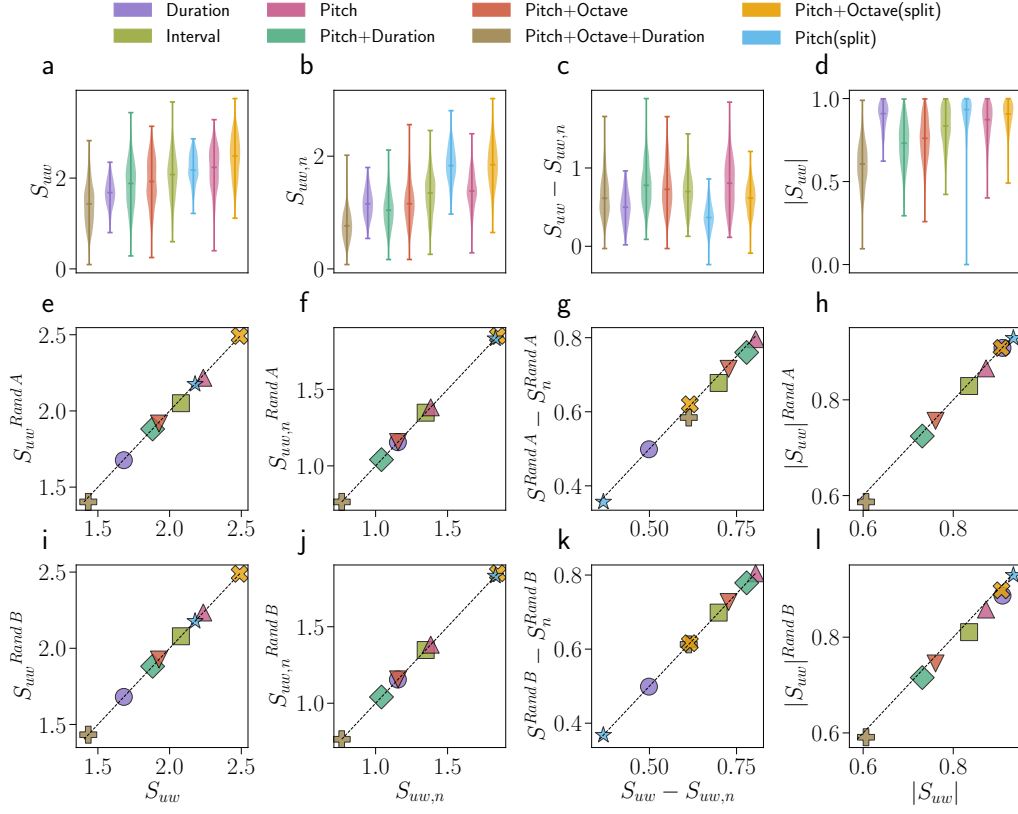

FIG. S15: Violin plots illustrating the distribution of (a) unweighted entropy  $S_{uw}$ , (b) average node unweighted entropy  $S_{uw,n}$ , (c) difference between unweighted entropy and average node unweighted entropy  $S_{uw} - S_{uw,n}$ , (d) normalized unweighted entropy  $|S_{uw}|$  for each network model. Each violin is color-coded by model, and the models are sorted by their mean unweighted entropy ( $S_{uw}$ ). The median of each distribution is indicated by a solid line within the violin. (e-l) The relationships between the median value of the original and randomized entropies. Two rows correspond to two types of network randomization (A and B). Here, we plot values for the left hand.

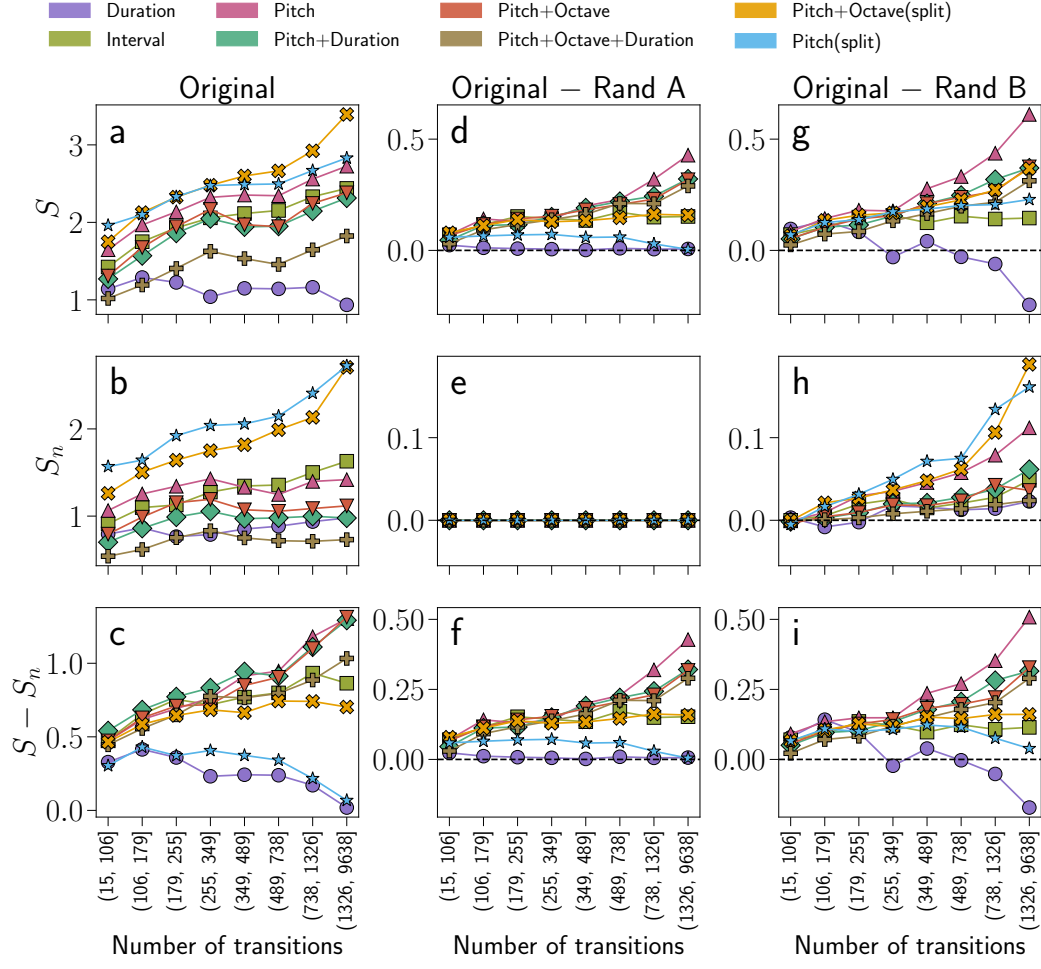

FIG. S16: The median values of entropy measures ((a) weighted entropy  $S$ , (b) average node weighted entropy  $S_n$ , (c) difference between weighted entropy and average node weighted entropy  $S - S_n$ ) split by the number of transitions. We bin the transition sizes into eight equally sized groups and compute the median values of entropy measures within each one. (d-i) The difference between the median value of entropy measures of the original and randomized network for each transition size bin. Two columns correspond to two types of network randomization (A and B). Here, we plot values for the left hand.

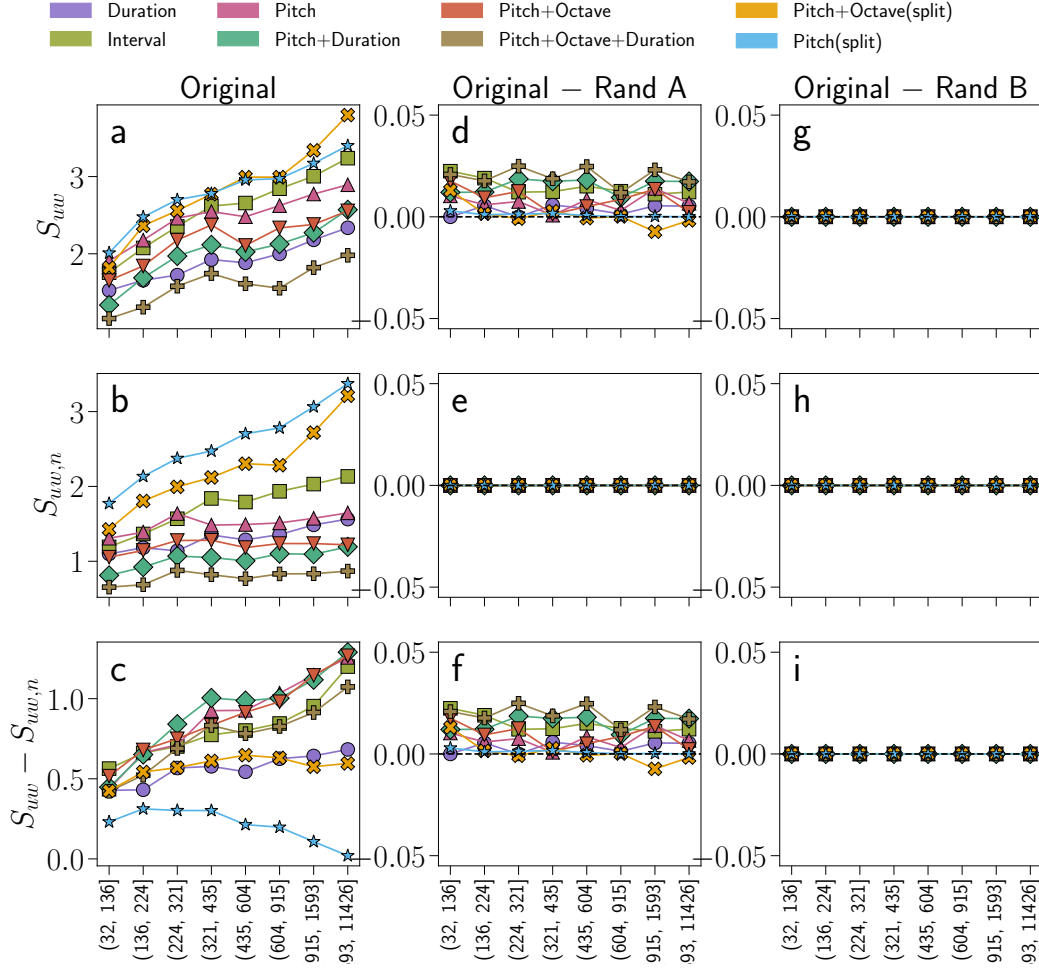

FIG. S17: The median values of entropy measures ((a) unweighted entropy  $S_{uw}$ , (b) average node unweighted entropy  $S_{uw,n}$ , (c) difference between unweighted entropy and average node unweighted entropy  $S_{uw} - S_{uw,n}$ ) split by the number of transitions. We bin the transition sizes into eight equally sized groups and compute the median values of entropy measures within each one. (d–i) The difference between the median value of entropy measures of the original and randomized network for each transition size bin. Two columns correspond to two types of network randomization (A and B). Here, we plot values for the right hand.

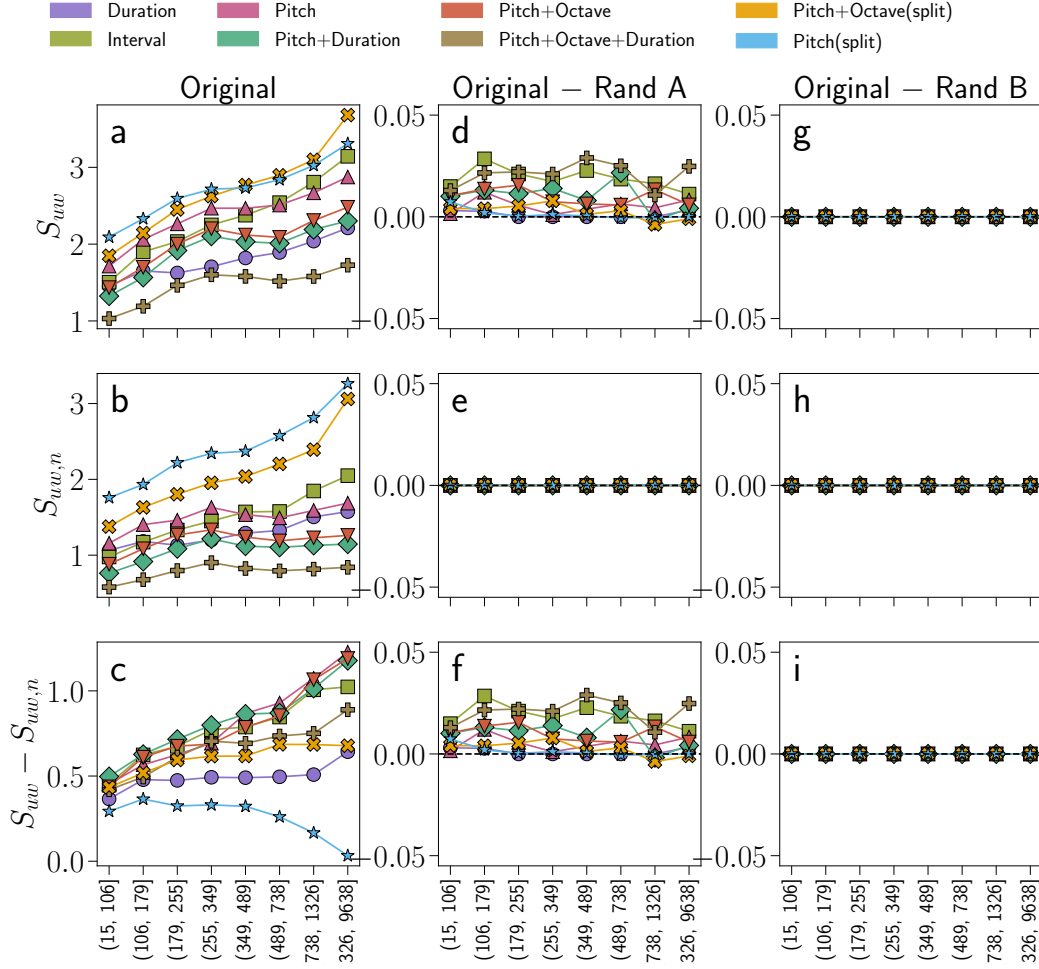

FIG. S18: The median values of entropy measures ((a) unweighted entropy  $S_{uw}$ , (b) average node unweighted entropy  $S_{uw,n}$ , (c) difference between unweighted entropy and average node unweighted entropy  $S_{uw} - S_{uw,n}$ ) split by the number of transitions. We bin the transition sizes into eight equally sized groups and compute the median values of entropy measures within each one. (d–i) The difference between the median value of entropy measures of the original and randomized network for each transition size bin. Two columns correspond to two types of network randomization (A and B). Here, we plot values for the left hand.



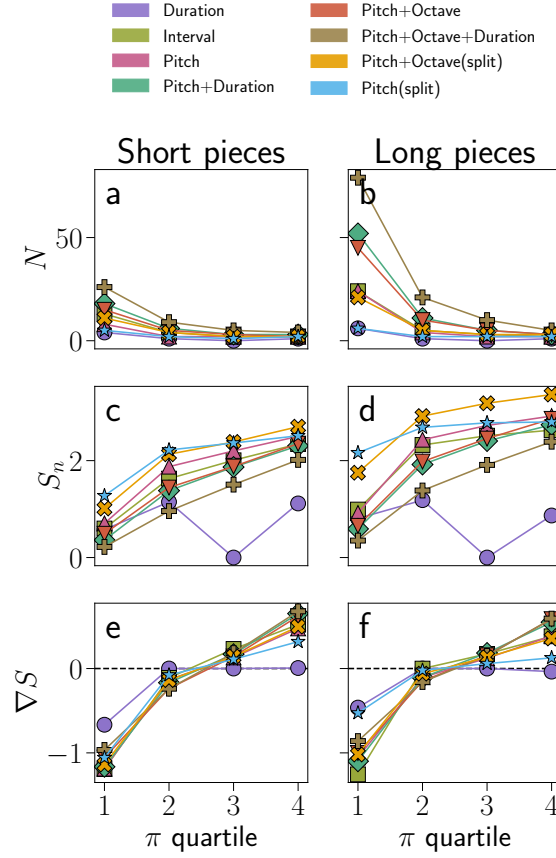

FIG. S19: The median values of (a, b) network size  $N$ , (c, d) average node weighted entropy  $S_n$ , and (e, f) gradient weighted entropy  $\nabla S$  for each quartile of the stationary distribution  $\pi$ . Two columns correspond to the short and long musical pieces. We grouped musical pieces by number of transitions into two equally sized bins. Here, we plot values for the left hand.

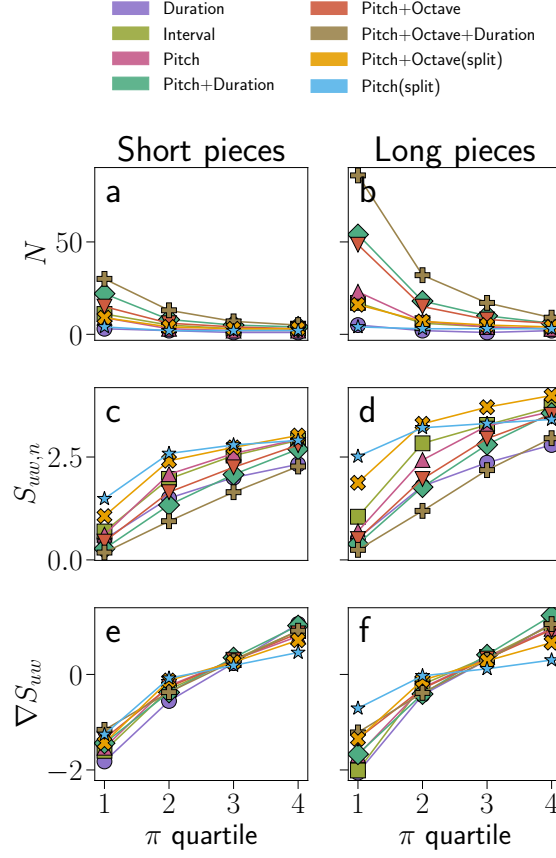

FIG. S20: The median values of (a, b) network size  $N$ , (c, d) average node unweighted entropy  $S_{uw,n}$ , and (e, f) gradient unweighted entropy  $\nabla S_{uw}$  for each quartile of the stationary distribution  $\pi$ . Two columns correspond to the short and long musical pieces. We grouped musical pieces by number of transitions into two equally sized bins. Here, we plot values for the right hand.

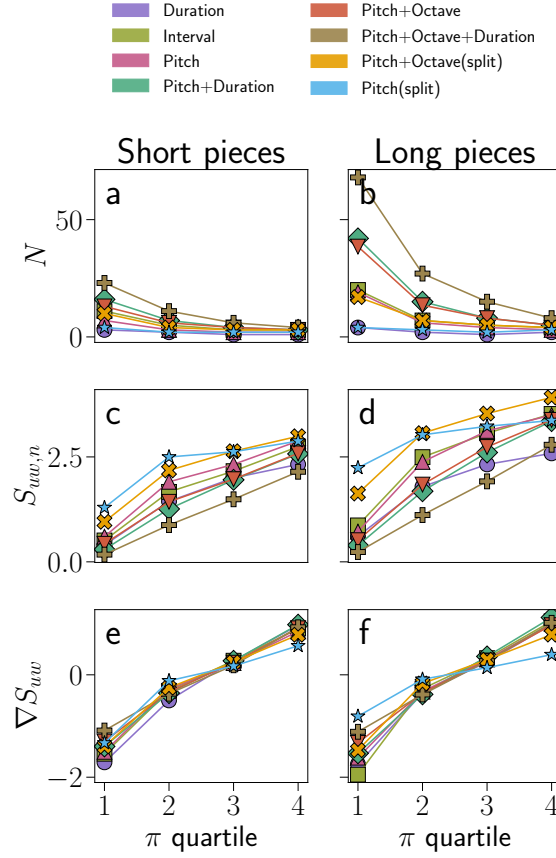

FIG. S21: The median values of (a, b) network size  $N$ , (c, d) average node unweighted entropy  $S_{uw,n}$ , and (e, f) gradient unweighted entropy  $\nabla S_{uw}$  for each quartile of the stationary distribution  $\pi$ . Two columns correspond to the short and long musical pieces. We grouped musical pieces by number of transitions into two equally sized bins. Here, we plot values for the left hand.

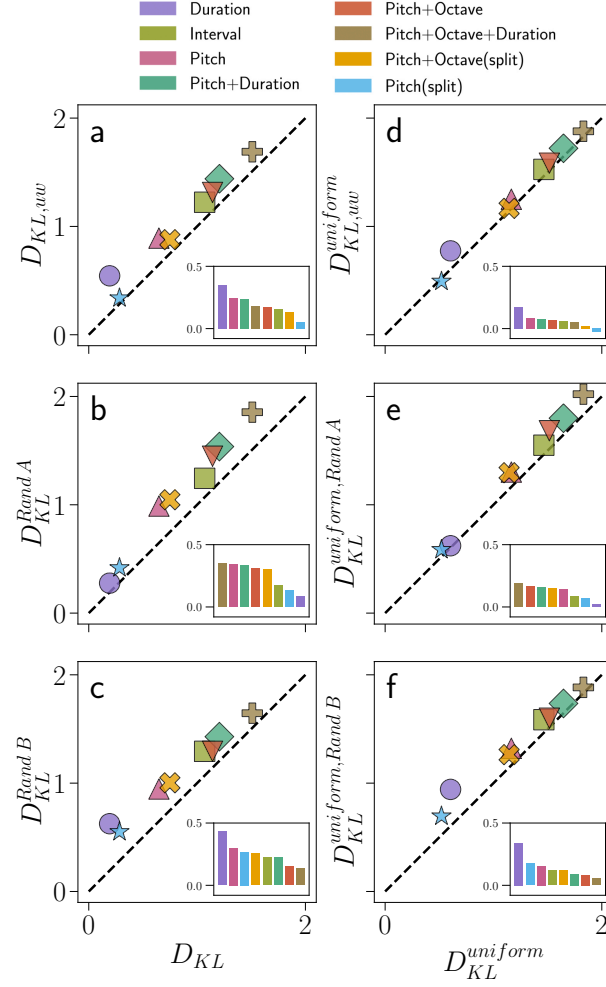

FIG. S22: The relationship between the median values of the original weighted, unweighted, and randomized Kullback-Leibler (KL) divergences. The first column corresponds to Eq. ??, whereas the second column corresponds to Eq. ?. (a, b) Difference in  $D_{KL}$  between weighted and unweighted networks. (b, e) Difference in  $D_{KL}$  between original weighted networks and after randomization A. (c, f) Difference in  $D_{KL}$  between original weighted networks and after randomization B. In each inset, the sorted difference per model is shown. We plot here the values for the left hand.

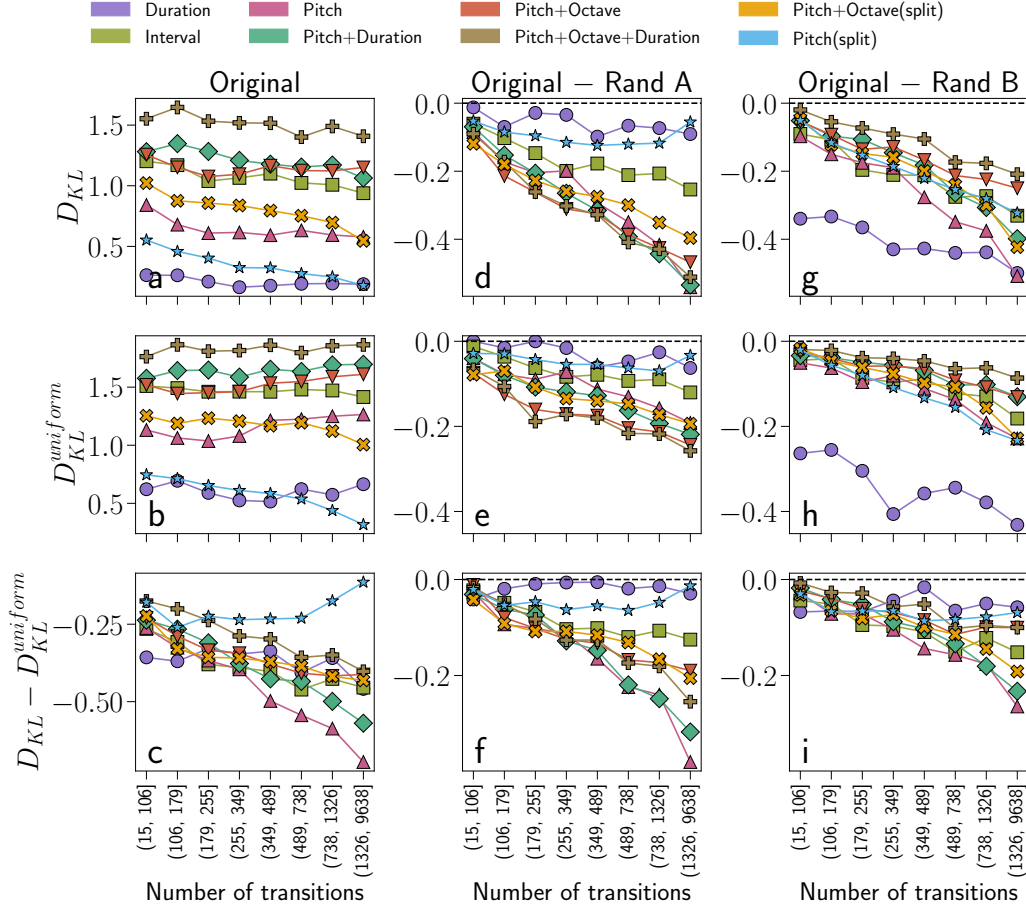

FIG. S23: The median values of divergence measures ((a) Kullback-Leibler (KL) divergence  $D_{KL}$ , (b) uniform Kullback-Leibler (KL) divergence  $D_{KL}^{uniform}$ , (c) difference  $D_{KL} - D_{KL}^{uniform}$ ) split by the number of transitions. We bin the transition sizes into eight equally sized groups and compute the median values of divergence measures within each one. (d-i) The difference between the median value of divergence measures of the original and randomized network for each transition size bin. Two columns correspond to two types of network randomization (A and B). Here, we plot values for the left hand.

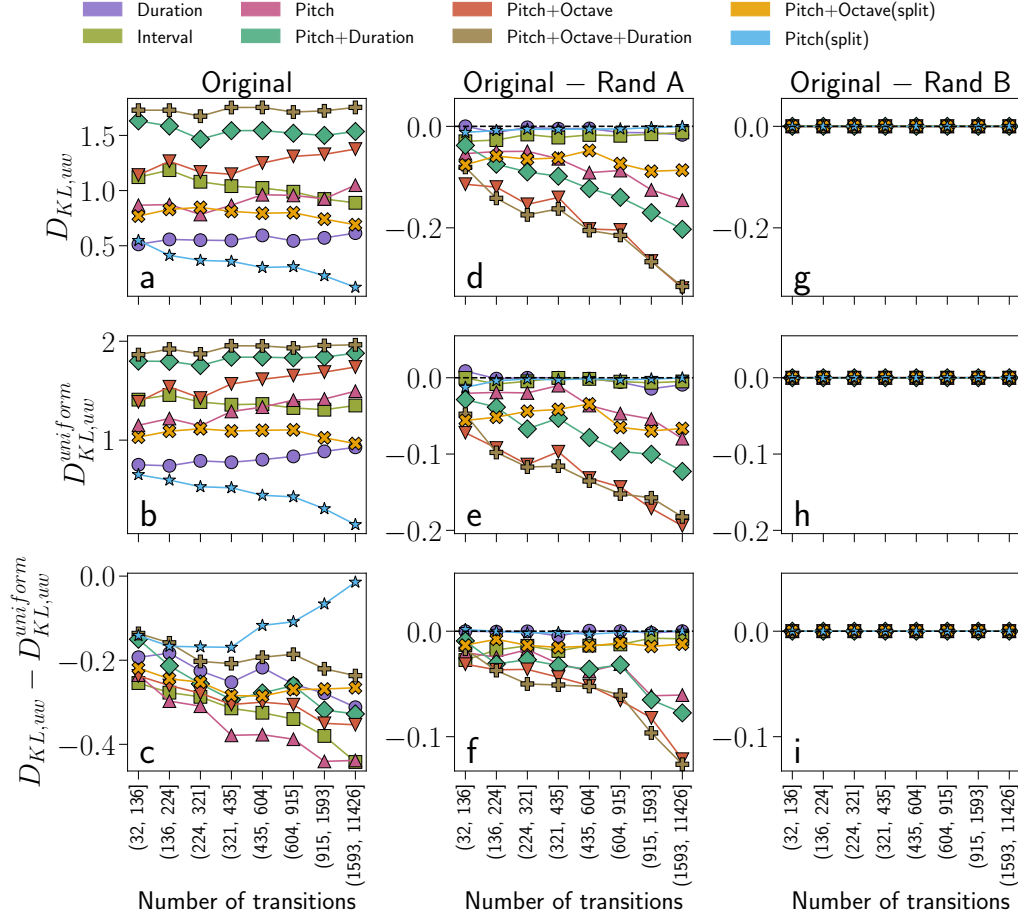

FIG. S24: The median values of divergence measures ((a) Kullback-Leibler (KL) divergence  $D_{KL}$ , (b) uniform Kullback-Leibler (KL) divergence  $D_{KL}^{uniform}$ , (c) difference  $D_{KL} - D_{KL}^{uniform}$ ) split by the number of transitions for the **unweighted** networks. We bin the transition sizes into eight equally sized groups and compute the median values of divergence measures within each one. (d-i) The difference between the median value of divergence measures of the original and randomized network for each transition size bin. Two columns correspond to two types of network randomization (A and B). Here, we plot values for the right hand.

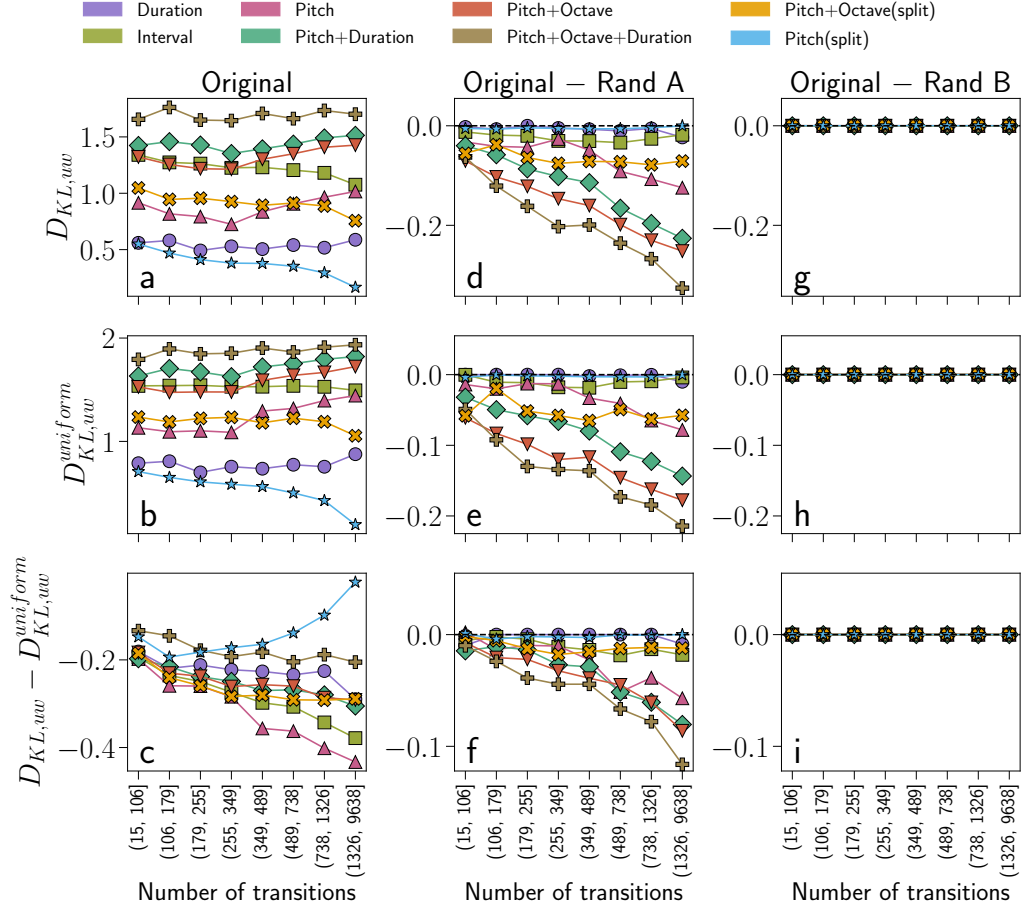

FIG. S25: The median values of divergence measures ((a) Kullback-Leibler (KL) divergence  $D_{KL}$ , (b) uniform Kullback-Leibler (KL) divergence  $D_{KL}^{uniform}$ , (c) difference  $D_{KL} - D_{KL}^{uniform}$ ) split by the number of transitions for the **unweighted** networks. We bin the transition sizes into eight equally sized groups and compute the median values of divergence measures within each one. (d-i) The difference between the median value of divergence measures of the original and randomized network for each transition size bin. Two columns correspond to two types of network randomization (A and B). Here, we plot values for the left hand.

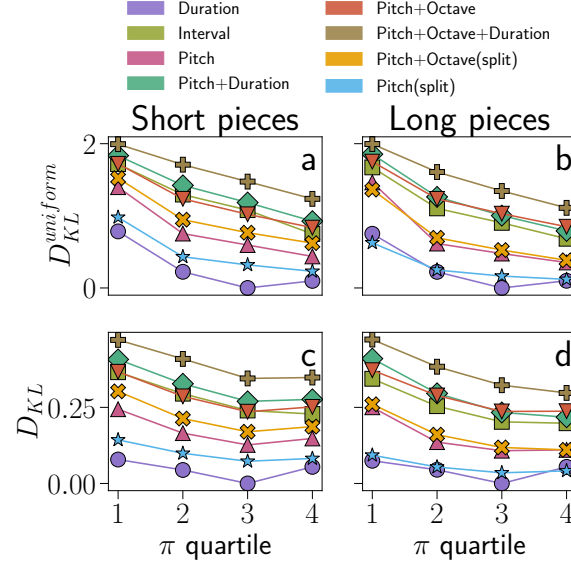

FIG. S26: The median values of (a, b) network size  $N$ , (c, d) uniform Kullback-Leibler divergence  $D_{KL}^{uniform}$ , and (e, f) Kullback-Leibler divergence  $D_{KL}$  for each quartile of the stationary distribution  $\pi$ . Two columns correspond to the short and long musical pieces. We grouped musical pieces by number of transitions into two equally sized bins. Here, we plot values for the left hand.

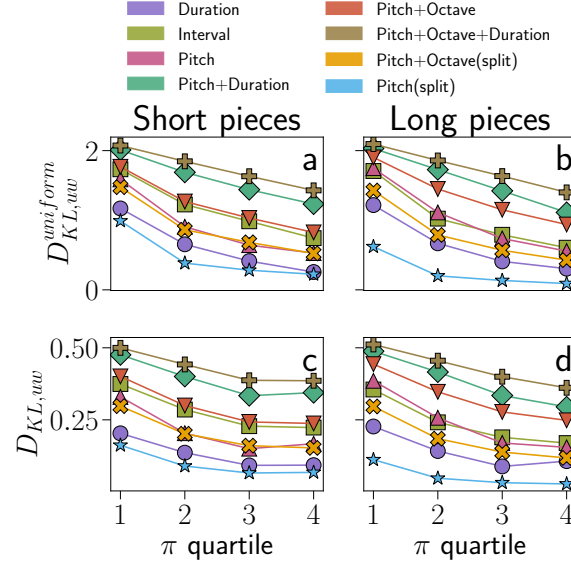

FIG. S27: The median values of (a, b) network size  $N$ , (c, d) uniform Kullback-Leibler divergence  $D_{KL}^{uniform}$ , and (e, f) Kullback-Leibler divergence  $D_{KL}$  for each quartile of the stationary distribution  $\pi$  for the **unweighted** networks. Two columns correspond to the short and long musical pieces. We grouped musical pieces by number of transitions into two equally sized bins. Here, we plot values for the right hand.



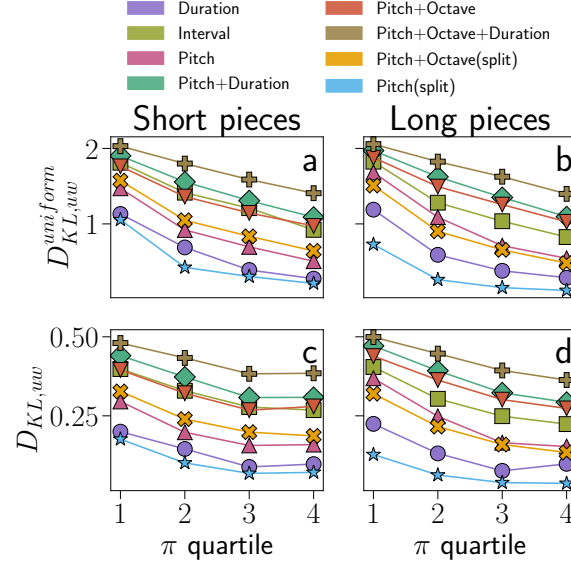

FIG. S28: The median values of (a, b) network size  $N$ , (c, d) uniform Kullback-Leibler divergence  $D_{KL}^{uniform}$ , and (e, f) Kullback-Leibler divergence  $D_{KL}$  for each quartile of the stationary distribution  $\pi$  for the **unweighted** networks. Two columns correspond to the short and long musical pieces. We grouped musical pieces by number of transitions into two equally sized bins. Here, we plot values for the left hand.
